# Supplementary material for: A Case for Fine-grain Coherence Specialization in Heterogeneous Systems
Source: arXiv:2104.11678 source file (2021-04-23)
Supplement: Supplementary file 1 [file appendix.tex]

\section{Appendix}
\label{sec:appendix}

\noindent 
\textbf{Program-conflict order} ($\xrightarrow{\text{pc}}$): In a sequentially consistent execution, program order is an ordering of accesses within the same thread, and conflict order is an ordering of accesses to the same address. Program-conflict order is the transitive closure of program order and conflict order, and forms a partial ordering of all accesses in the sequentially consistent execution.

\noindent 
\textbf{Reuse window (Appendix)}: \textbf{reuseWindow}($A$) returns a set of memory accesses surrounding $A$ from the issuing device $D$ during which the cache block accessed by $A$ is unlikely to have been evicted. For simplicity, we define this as all accesses $B$ from $D$ which satisfy the following constraints:

\begin{enumerate}
    \item $B \not\xrightarrow{\text{pc}} A$.
    \item For all accesses $C_i$ that satisfy $C_i \not\xrightarrow{\text{pc}} A$ and $C_i \xrightarrow{\text{pc}} B$, the total number of unique bytes accessed by all $C_i$ is less than some value $N$. We choose $N$ to be 75\% the capacity of the local cache.
\end{enumerate}
